# Supplementary material for: Demystifying Invariant Effectiveness for Securing Smart Contracts
Source: arXiv:2404.14580 source file (2024-07-14)
Supplement: Supplementary file 1 [file FlashSyn.tex]

\subsection{From FlashSyn}

\textbf{Eminence}

Protocol Type: yield-earning

Vulnerability Type: logic flaw

Victim Contract: 
0x5ade7aE8660293F2ebfcEfaba91d141d72d221e8

Hack Tx:
0x3503253131644dd9f52802d071de74e456570374d586ddd640159cf6fb9b8ad8

\textbf{Harvest\_fUSDT}

Protocol Type: yield-earning

Vulnerability Type: Oracle manipulation

Victim Contract: 
0x053c80ea73dc6941f518a68e2fc52ac45bde7c9c

Implementation:
0x9b3be0cc5dd26fd0254088d03d8206792715588b

Hack Tx:
0x3503253131644dd9f52802d071de74e456570374d586ddd640159cf6fb9b8ad8

\textbf{Harvest\_fUSDC}

Protocol Type: yield-earning

Vulnerability Type: Oracle manipulation

Victim Contract: 
0xf0358e8c3cd5fa238a29301d0bea3d63a17bedbe

Implementation:
0x9b3be0cc5dd26fd0254088d03d8206792715588b

Hack Tx:
0x35f8d2f572fceaac9288e5d462117850ef2694786992a8c3f6d02612277b0877

\textbf{ValueDeFi}

Protocol Type: yield-earning

Vulnerability Type: Oracle manipulation

Comments: Actually they implemented depositCap

Victim Contract:
0x55BF8304C78Ba6fe47fd251F37d7beb485f86d26

Implementation:
0xddd7df28b1fb668b77860b473af819b03db61101

Hack Tx:
0x46a03488247425f845e444b9c10b52ba3c14927c687d38287c0faddc7471150a

\textbf{Yearn}

Protocol Type: yield-earning

Vulnerability Type: Logic flaw, Force investment

Victim Contract: StrategyDAI3pool
0x9c211bfa6dc329c5e757a223fb72f5481d676dc1

Hack Tx:
0xf6022012b73770e7e2177129e648980a82aab555f9ac88b8a9cda3ec44b30779

\textbf{bZx2}

Protocol Type: Multiple tokens, lending protocols

Vulnerability Type: reentrancy + manipulation

Victim Contract:
0x77f973FCaF871459aa58cd81881Ce453759281bC

implementation:
0x85ca13d8496b2d22d6518faeb524911e096dd7e0

Hack Tx:
0x762881b07feb63c436dee38edd4ff1f7a74c33091e534af56c9f7d49b5ecac15

\textbf{Warp}  good lending
Victim Contract: DAI
0x6046c3Ab74e6cE761d218B9117d5c63200f4b406

Victim Contract: USDC (have not collected)
0xae465fd39b519602ee28f062037f7b9c41fdc8cf

Hack Tx:
0x8bb8dc5c7c830bac85fa48acad2505e9300a91c3ff239c9517d0cae33b595090

\textbf{CheeseBank}    good  lending 
Victim Contract:
sUSDC
0x5E181bDde2fA8af7265CB3124735E9a13779c021
sUSDT
0x4c2a8A820940003cfE4a16294B239C8C55F29695
sDAI
0xA80e737Ded94E8D2483ec8d2E52892D9Eb94cF1f

Hack Tx:
0x600a869aa3a259158310a233b815ff67ca41eab8961a49918c2031297a02f1cc

\textbf{InverseFi} good  lending 
Victim Contract:
0x7Fcb7DAC61eE35b3D4a51117A7c58D53f0a8a670

Hack Tx:
0x958236266991bc3fe3b77feaacea120f172c0708ad01c7a715b255f218f9313c

\textbf{bZx1} 

This case is dropped because the victim contracts are close source. 

Victim Contract:
0xb0200B0677dD825bb32B93d055eBb9dc3521db9D

 unfortunately the contracts are close-source
<!-- 0xb017c9936f9271daff23d4c9876651442958a80f -->

Hack Tx:
0xb5c8bd9430b6cc87a0e2fe110ece6bf527fa4f170a4bc8cd032f768fc5219838
