# Supplementary material for: Demystifying Invariant Effectiveness for Securing Smart Contracts
Source: arXiv:2404.14580 source file (2024-07-14)
Supplement: Supplementary file 2 [file GitHub.tex]

\subsection{From GitHub}

DeFi hacks Victim Contract List
Victim Contract is defined as the contracts which transfer out financial losses.

\textbf{Opyn} 
Victim Contract: 
0x951d51baefb72319d9fbe941e1615938d89abfe2

Transaction History Len:
107

Hack Tx:
0x56de6c4bd906ee0c067a332e64966db8b1e866c7965c044163a503de6ee6552a

\textbf{Cover Protocol} Dropped because 

Mint tons of cover tokens  16453
Victim Contract:
<!-- 0xe0b94a7bb45dd905c79bb1992c9879f40f1caed5 -->

(Have to give up because there is no profit)
Hack Tx:
<!-- 0xca135d1c4268d6354a019b66946d4fbe4de6f7ddf0ff56389a5cc2ba695b035f -->

20210509 RariCapital - Cross Contract Reentrancy  54318

Victim Contract:
0x67b66c99d3eb37fa76aa3ed1ff33e8e39f0b9c7a

Hack Tx:
0x171072422efb5cd461546bfe986017d9b5aa427ff1c07ebe8acc064b13a7b7be

20210702 Chainswap - Bridge, logic flaw
close source

20210830 Cream Finance - Flashloan Attack + Reentrancy

Victim Contract:
(Cream.Finance: crAMP Token) Borrow 223
0x3c710b981f5ef28da1807ce7ed3f2a28580e0754  
 (Cream.Finance: crETH Token) Borrow 62358
0xd06527d5e56a3495252a528c4987003b712860ee 

Hack Tx:
0xa9a1b8ea288eb9ad315088f17f7c7386b9989c95b4d13c81b69d5ddad7ffe61e

20210915 NowSwap Platform

Victim Contract:
Close source

Hack Tx:

## 20211015 Indexed Finance - protocol valuation Manipulation 20946
Very very complicated

Uniswap Protocol: UNI token

Aave: AAVE Token

Compound: COMP Token

Curve.fi: CRV Token

Victim Contract:
0x5bd628141c62a901e0a83e630ce5fafa95bbdee4

Hack Tx:
0x44aad3b853866468161735496a5d9cc961ce5aa872924c5d78673076b1cd95aa

## 20211027 CreamFinance - Price Manipulation
Victim Contract:

Cream.Finance: crUSDC Token  63769   borrow
0x44fbebd2f576670a6c33f6fc0b00aa8c5753b322

<!-- Cream.Finance: crETH Token 62358 borrow -->
<!-- 0xd06527d5e56a3495252a528c4987003b712860ee -->

Cream.Finance: crUSDT Token 42909 borrow
0x797aab1ce7c01eb727ab980762ba88e7133d2157

Cream.Finance: crUNI Token 18078 borrow
0xe89a6d0509faf730bd707bf868d9a2a744a363c7

Cream.Finance: crFEI Token 213 borrow
0x8c3b7a4320ba70f8239f83770c4015b5bc4e6f91

XXX and several small tokens

Hack Tx:
0x0fe2542079644e107cbf13690eb9c2c65963ccb79089ff96bfaf8dced2331c92

## 20211221 Visor Finance - Reentrancy  
Victim Contract: 3283
0xc9f27a50f82571c1c8423a42970613b8dbda14ef

Hack Tx:
0x6eabef1bf310a1361041d97897c192581cd9870f6a39040cd24d7de2335b4546

## 20220320 Umbrella Network - Underflow Lost: $700k    
Victim Contract:  111
0xb3fb1d01b07a706736ca175f827e4f56021b85de

Hack Tx:
0x33479bcfbc792aa0f8103ab0d7a3784788b5b0e1467c81ffbed1b7682660b4fa

## Revest Finance - Reentrancy But it's related to token flow analysis
Victim Contract: 1671
0xa81bd16aa6f6b25e66965a2f842e9c806c0aa11f

Hack Tx:
0xe0b0c2672b760bef4e2851e91c69c8c0ad135c6987bbf1f43f5846d89e691428

<----> 0x56de8bc61346321d4f2211e3ac3c0a7f00db9b76 transfer

## 20220329 Ronin Network - Bridge
Victim Contract: ETH    3081122 txs
0x8407dc57739bcda7aa53ca6f12f82f9d51c2f21e

Hack Tx:  
0xc28fad5e8d5e0ce6a2eaf67b6687be5d58113e16be590824d6cfa1a94467d0b7

Victim Contract: USDC   3081122 txs
0x8407dc57739bcda7aa53ca6f12f82f9d51c2f21e

Hack Tx:
0xed2c72ef1a552ddaec6dd1f5cddf0b59a8f37f82bdda5257d9c7c37db7bb9b08

## 20220416 BeanstalkFarms - DAO + Flashloan
Victim Contract:  emergencyCommit 
<!-- 0xc1e088fc1323b20bcbee9bd1b9fc9546db5624c5 -->

<!-- implementation: UNI-V2 transfer     309 --> Minimum  neglectable
<!-- 0xf480ee81a54e21be47aa02d0f9e29985bc7667c4 -->

Victim Contract: BEAN3CRV-f remove_liquidity_one_coin   3Crv.transfer    6311
0x3a70dfa7d2262988064a2d051dd47521e43c9bdd

Victim Contract:  BEANLUSD-f remove_liquidity_one_coin   LUSD.transfer  322
0xd652c40fbb3f06d6b58cb9aa9cff063ee63d465d   

Hack Tx:
0xcd314668aaa9bbfebaf1a0bd2b6553d01dd58899c508d4729fa7311dc5d33ad7

## 20220430 Rari Capital/Fei Protocol - Flashloan Attack + Reentrancy

Victim Contract  fETH-127  borrow   694
0x26267e41ceca7c8e0f143554af707336f27fa051

Victim Contract   fUSDC-127 borrow   905
0xebe0d1cb6a0b8569929e062d67bfbc07608f0a47

Victim Contract    USDT    472
0xe097783483d1b7527152ef8b150b99b9b2700c8d

Victim Contract   frax     852
0x8922c1147e141c055fddfc0ed5a119f3378c8ef8

Hack Tx:
0xab486012f21be741c9e674ffda227e30518e8a1e37a5f1d58d0b0d41f6e76530

## 20220430 Saddle Finance - Swap Metapool Attack

Victim Contract: 
<!-- 0xacb83e0633d6605c5001e2ab59ef3c745547c8c7 -->
DAI:0x6b175474e89094c44da98b954eedeac495271d0f
USDC:0xa0b86991c6218b36c1d19d4a2e9eb0ce3606eb48
USDT:0xdac17f958d2ee523a2206206994597c13d831ec7
Implementation: 19310   SwapUtils
0x2069043d7556b1207a505eb459d18d908df29b55

Hack Tx:
0x2b023d65485c4bb68d781960c2196588d03b871dc9eb1c054f596b7ca6f7da56

## 20220624 Harmony's Horizon Bridge - Private key compromised  (could be ignored)

Victim Contract:   40261
0xf9fb1c508ff49f78b60d3a96dea99fa5d7f3a8a6

Hack Tx:
0x27981c7289c372e601c9475e5b5466310be18ed10b59d1ac840145f6e7804c97

## 20220626 XCarnival - Infinite Number of Loans

Victim Contract:
<!-- 0xb38707e31c813f832ef71c70731ed80b45b85b2d -->

Implementation:  ether transfer   344
0x5417da20ac8157dd5c07230cfc2b226fdcfc5663

Hack Tx:
0x51cbfd46f21afb44da4fa971f220bd28a14530e1d5da5009cfbdfee012e57e35

(learn-evm-attacks)
## Jan 19, 2022 Multichain Permit Attack  AnySwap  
Victim Contract: which eventually transfers Ether to the exploiter   123046  
0x6b7a87899490EcE95443e979cA9485CBE7E71522

Hack Tx:
0xe50ed602bd916fc304d53c4fed236698b71691a95774ff0aeeb74b699c6227f7

(learn-evm-attacks)
## Furucombo
## Total lost: ~$15MM USD (in different tokens)
## steal from users

(learn-evm-attacks)
## Nomad bridge Date: Aug 1, 2022
Victim Contract:   46955
0x88a69b4e698a4b090df6cf5bd7b2d47325ad30a3

Hack Tx:
0xa5fe9d044e4f3e5aa5bc4c0709333cd2190cba0f4e7f16bcf73f49f83e4a5460

(learn-evm-attacks)
## PolyNetwork Bridge, Aug 2021
Victim Contract:   54961
0x250e76987d838a75310c34bf422ea9f1ac4cc906

Hack Tx:
0xad7a2c70c958fcd3effbf374d0acf3774a9257577625ae4c838e24b0de17602a

########## Access Control

## Pickle Finance Access Control  cDAI

Victim Contract: 6041  ControllerV4
0x6847259b2B3A4c17e7c43C54409810aF48bA5210

Hack Tx:
0xe72d4e7ba9b5af0cf2a8cfb1e30fd9f388df0ab3da79790be842bfbed11087b0

## DODO  Access Control, init  
Victim Contract:  1796
0x2bbd66fc4898242bdbd2583bbe1d76e8b8f71445

Hack Tx:
0x395675b56370a9f5fe8b32badfa80043f5291443bd6c8273900476880fb5221e

## 20210903 DAO Maker - Bad Access Control
Victim Contract:
Close Source

Hack Tx:
<!-- 0xd5e2edd6089dcf5dca78c0ccbdf659acedab173a8ab3cb65720e35b640c0af7c -->

## 20220214 BuildFinance - DAO  Access Control 
Victim Contract:  51289
0x6e36556b3ee5aa28def2a8ec3dae30ec2b208739

Hack Tx:
0x544e5849b71b98393f41d641683586d0b519c46a2eeac9bcb351917f40258a85

## 20220305 Bacon Protocol - Reentrancy
Victim Contract:   1167
0xb8919522331c59f5c16bdfaa6a121a6e03a91f62

Hack Tx:
0x7d2296bcb936aa5e2397ddf8ccba59f54a178c3901666b49291d880369dbcf31

(learn-evm-attacks)

## Punk Protocol Re-initialize Aug 10, 2021
Victim Contract:  
Punk USDC: 31
0x3BC6aA2D25313ad794b2D67f83f21D341cc3f5fb

Punk USDT: 46
0x1F3b04c8c96A31C7920372FFa95371C80A4bfb0D

Punk DAI:  40
0x929cb86046E421abF7e1e02dE7836742654D49d6

Hack Tx: WhiteHat Hack
0x597d11c05563611cb4ad4ed4c57ca53bbe3b7d3fefc37d1ef0724ad58904742b
