# Supplementary material for: Demystifying Invariant Effectiveness for Securing Smart Contracts
Source: arXiv:2404.14580 source file (2024-07-14)
Supplement: Supplementary file 3 [file invariants.tex]

\section{Risk Management Invariants}

This section lists all the invariants we collected from various sources.
We categorize these invariants into different categories based on the protocols 
they were applied to.

sources:

\label{src:dforce} dForce, audited by ConsenSys, Trail of Bits, Certora, Certik 

\label{src:euler} Euler, audited by Solidified and ZK Labs, Halborn, Certora, Sherlock, Omniscia

\label{src:aave} AAVE, audited by SigmaPrime, Certora, Peckshield, ABDK, SigmaPrime, Certora, Peckshield, Trail of Bits, OpenZeppelin

\label{src:uniswapV3} uniswapV3, audited by Trail of Bits, ABDK, samczsun

\label{audit:fei} Fei's ConsenSys' audit report \href{https://consensys.net/diligence/audits/2021/09/fei-protocol-v2-phase-1/}.

\label{audit:SolidityFi} Solidity Finance's OKLG's audit report \href{https://solidity.finance/audits/OKLG/}.

\label{blog:hacken} Hacken's blog post on How to prevent smart contract vulnerabilities \href{https://hacken.io/discover/smart-contract-vulnerabilities/#4_Flashloan_Attack_High}.`'

\label{audit:eigenlayer} ConsenSys' auditing reports on EigenLayer \href{https://consensys.io/diligence/audits/2023/03/eigenlabs-eigenlayer/}.

\label{audit:mStable} ConenSys' auditing reports on mStable \href{https://consensys.io/diligence/audits/2020/07/mstable-1.1/#swap-fees-can-be-bypassed-using-redeemmasset}.
 
\label{src:idle} Idle Finance audited by Quantstamp, ConsenSys. \href{https://docs.idle.finance/}. 

\subsection{Lending Protocols}

\subsubsection{Supply Capacity for an asset}
The maximum supplying amount of collateral. If the capacity meets, no more supply is permitted.

/*
*  The supply capacity of the asset, will be checked in beforeMint()
*  -1 means there is no limit on the capacity
*  0 means the asset can not be supplied any more
*/

sources: \ref{src:dforce}.

Supply caps define the maximum amount of an asset which can be supplied to the protocol. Supply caps can be used to limit the protocol’s exposure to riskier assets and protect against infinite minting exploits. A supply cap is an optional parameter, and the value will depend on on-chain liquidity of the asset and total volume of collateral assets in the pool.

sources: \ref{src:aave}.

\subsubsection{Borrow Capacity for an asset}
The maximum borrowing amount of borrow asset. If the capacity meets, no more borrows are permitted.

/*
*  The borrow capacity of the asset, will be checked in beforeBorrow()
*  -1 means there is no limit on the capacity
*  0 means the asset can not be borrowed any more
*/

sources: \ref{src:dforce}.

Borrow caps define the maximum amount of an asset which can be borrowed. Borrow caps can be used to prevent traditional and flash borrowing of an asset which may experience a price exploit and lead to protocol insolvency. A borrow cap is an optional parameter, and the value will depend on-chain liquidity of the asset and total volume of borrowed assets in the pool.

sources: \ref{src:aave}.

\subsubsection{Borrow range for a user}

Minimum Borrow Balance
This function returns the minimum borrow balance allowed in the base asset. An account’s initial borrow size must be equal to or greater than this value. Subsequent borrows may be of any size.

\subsubsection{Asset Tiers}

Assets fall into three different tiers: isolated, cross and collateral tiers.

Isolated tier assets are available for ordinary lending and borrowing, but they cannot be used as collateral to borrow other assets, and they can only be borrowed in isolation. What this means is that they cannot be borrowed alongside other assets using the same pool of collateral. For example, if a user has USDC and DAI as collateral, and they want to borrow isolation-tier asset ABC, then they can only borrow ABC. If they later want to borrow another token, XYZ, then they can only do so using a separate account on Euler.

Cross tier assets are available for ordinary lending and borrowing, and cannot be used as collateral to borrow other assets, but they can be borrowed alongside other assets. For example, if a user has USDC and DAI as collateral, and they want to borrow cross-tier assets ABC and XYZ, then they can do so from a single account on Euler.

Collateral tier assets are available for ordinary lending and borrowing, cross-borrowing, and they can be used as collateral. For example, a user can deposit collateral assets DAI and USDC, and use them to borrow collateral assets UNI and LINK, all from a single account. \

sources: \ref{src:euler}.

Isolation mode can be used to limit the systemic risk of listing riskier assets. Isolation mode limits an asset to only borrow isolated stablecoins and only use a single isolated asset as collateral at a time. More info on isolation mode can be found here.

Siloed Mode
In V3, new assets with potentially manipulatable oracles (e.g., illiquid Uni V3 pairs where the price can be affected drastically by a single trade) can be listed in Siloed Mode to limit the overall risk of insolvency of the protocol. A siloed asset on the Aave Protocol restricts the borrower to single borrows only (i.e., a user borrowing a siloed asset cannot borrow any other asset).

eMode
Efficient Mode (”eMode”) allows assets which are correlated in price (e.g., DAI, USDC, and USDT) to be listed in the same eMode category which maximises capital efficiency by allowing higher LTVs when both the borrowed and collateral asset belong to the same eMode category. Currently, only a single eMode category is defined in the Aave Protocol V3 markets - Stablecoins, category 1.

\subsection{Yield Earning Protocols}

\subsubsection{Minimum Shares(to prevent donation attacks)}

EigenLabs Quick Summary: The StrategyBase contract sets a minimum initial deposit amount of 1e9. This is to mitigate ERC-4626 related inflation attacks, where an attacker can front-run a deposit, inflating the exchange rate between tokens and shares. A consequence of that protection is that any amount less than 1e9 is not withdrawable.

// Calculate the value that `totalShares` will decrease to as a result of the withdrawal

// check to avoid edge case where share rate can be massively inflated as a 'griefing' sort of attack

\subsection{All types}

\subsubsection{balanceOf checks}

token flow compared with balanceOf(address(this)).

$ IERC20(_mAsset).balanceOf(address(this)) >= interestCollected + newReward $

sources: \href{https://github.com/mstable/mStable-contracts/blob/master/contracts/savings/SavingsManager.sol}.

\subsubsection{Timelocks}

Deposit and Withdraw must be timelocked for some time. 
sources: \ref{blog:hacken} \ref{src:idle}

Cannot deposit twice in 6 hours. 
sources: \href{https://github.com/mstable/mStable-contracts/blob/master/contracts/savings/SavingsManager.sol}.

// Ensures no actor can change the pool contents earlier in the block
require(lastChangeBlock < block.number, "BalancerLBPSwapper: pool changed this block");

sources: \ref{audit:fei}

\subsubsection{Re-entrancy}

It's been studied generally by prior work. 

the practice of the check-effect-interaction

https://fravoll.github.io/solidity-patterns/checks_effects_interactions.html

The Solidity documentation suggests that require() “should be used to ensure valid conditions, such as inputs, or contract state variables [..], or to validate return values from calls to external contracts” and assert() “should only be used to test for internal errors, and to check invariants”. Both methods evaluate the parameters passed to it as a boolean and throw an exception if it evaluates to false. The revert() throws in every case. It is therefore useful in complex situations, like if-else trees, where the evaluation of the condition can not be conducted in one line of code and the use of ‘require()’ would not be fitting.

http://solidity.readthedocs.io/en/v0.4.21/#

\subsubsection{Access Control}

It's been studied generally by prior work.

\subsubsection{Slippage Control}
Slippage simply means the difference between the price that you see on the screen when initialing a transaction and the actual price the swap is executed at.

It could be applied to anywhere involving an oracle price and not just DEX. 

sources: \ref{src:uniswapV3}.

\subsubsection{Oracle Price Assumption}

\subsubsection{Result value must be constant or non-zero}

sources: \ref{audit:mStable}.

\subsubsection{msg.sender and tx.origin}

msg.sender must be a contract.

\subsubsection{Inputs}
input parameter (integer) must be smaller than some constants, for example, totalShares

input parameter must be equal to some constants, for example, 0

\subsubsection{Outputs}

Intermediate states != a constant

Poststates must be bigger than a constant

% initialBalance == finalBalance

% A function’s return value must be some values

% A return value of a function must == some value
%    if (order.maker != msg.sender) revert AccessDenied();

%     orderHash = hashOrder(order);
%     orderRemaining = _remaining[orderHash];
%     if (orderRemaining == _ORDER_FILLED) revert AlreadyFilled();

% require(success);

% X (address) != 0x0
% X (address) == msg.sender

% X > constant 

% Msg.sender != XXX
% Msg.value == function

% assembly {
%     codeSize := extcodesize(_target)
% }
% require(codeSize > 0);

% Intermediate calculation < constant

% X.address != constant
% sload aa == sload bb

deposit Cap:  ValueDeFi

\subsection{gas}

https://github.com/OokiTrade/contractsV2/blob/4fafa4c2f142753ca0492914d171b6b774af5c6d/contracts/helpers/HelperProxy.sol#L30

Invariant Combination 

https://vscode.blockscan.com/arbitrum-one/0x42efe3e686808cca051a49bcde34c5cba2ebefc1

https://arbiscan.io/address/0x42efe3e686808cca051a49bcde34c5cba2ebefc1#code#F19#L108

GMX cooldown
