# Supplementary material for: Demystifying Invariant Effectiveness for Securing Smart Contracts
Source: arXiv:2404.14580 source file (2024-07-14)
Supplement: Supplementary file 4 [file appendix.tex]

\input{tables/RQ1.tex}

\begin{figure}[h]
	\centering
	\includegraphics[width=0.8\textwidth]{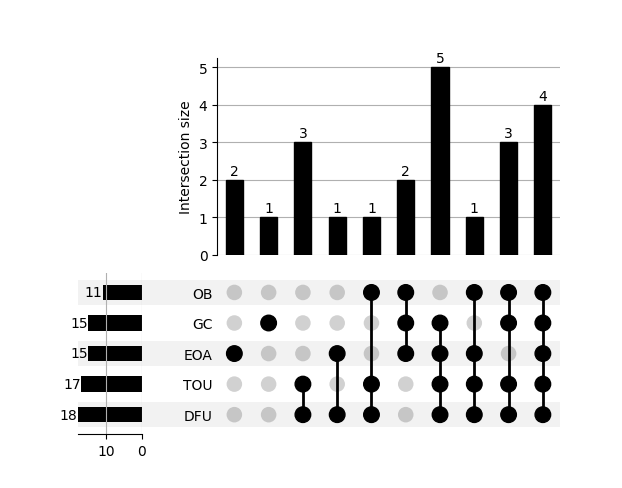}
	\vspace{-5mm}
	\caption{Upset Plot of Distinct Intersections of Invariants' Blocked Hacks}
	\label{fig:distinctHacks}
\end{figure}

To facilitate this analysis, we employ an upset plot to compare sets of hacks blocked by each invariant, as illustrated in Figure~\ref{fig:distinctHacks}. An upset plot visualizes the size of each distinct intersection set among the data sets being compared. The intersection set with size 0 is ignored. It is particularly useful for showing how different data sets overlap or diverge in terms of shared elements. In this context, it allows us to identify which exploits are uniquely blocked by individual invariants and how various invariants perform in combination. We observe that some invariants are strictly stronger than others; for example, DFU is shown to be strictly stronger than TOU because it can block all hacks that TOU can, plus more. For example, there are two exploits that can only be blocked by onlyEOA invariant(the first column). No exploits can only be blocked by OB, TOU or DFU, as they have no columns. There are 4 exploits that can be blocked by each of the five invariants(last column). We also find that DFU is more robust than TOU, capturing all the exploits that TOU can block.

\section{Harvest Vault Hack Case Study}

On October 26, 2020, USDC and USDT vaults of the Harvest Finance were exploited, causing a
financial loss of about USD \$$33.8$ million.
The first exploit transaction to the USDC vault from this attack provides a strong motivation to
this research.
The exploit transaction contains a sequence of function calls that interact with the following
smart contracts:

\begin{itemize}
  \item \textbf{Attack Contract:} The attack contract is a contract deployed by the attacker to
  execute the complex logic of the attack.
  It also serves as the callee of the flash loan. \yi{what is a flashloan?}
  Namely, the flash loan provider will execute a certain function within the attack contract with
  flash loan. It enables the hacker to execute complicated logic within a single transaction.
  \item \textbf{Harvest Vault Contract:} Harvest vault contract is the main user interface contract of Harvest Finance Protocol. It is the victim contract of this attack. Users can deposit USDC into this vault contract and receive fUSDC tokens. Users can later use fUSDC tokens to retrieve their deposit back. The conversion rate of fUSDC and USDC is determined by current USDC balance of the vault contract, an external call \codeword{investedUnderlyingBalance()} to Harvest Strategy Contract, and the total supply of fUSDC tokens.
  \item \textbf{Harvest Strategy Contract:} Harvest strategy contract is a contract that implements the investment strategy of Harvest Finance. It has a read-only function \codeword{investedUnderlyingBalance()} that calculates and returns the estimate of invested assets. However, the return value could be manipulated as this function uses the balances of Curve Y Pool contract to calculate the estimate.
  \item \textbf{Curve.Fi Y Pool Contract} Curve.Fi is an exchange protocol for stable coins. Curve.Fi Y pool contract maintains a pool of DAI, USDC, USDT, and TUSD. Users can exchange one kind of stable coins to another in this pool. The exchange rate is determined by the current balances of DAI, USDC, USDT, and TUSD in the pool. However, hackers can manipulate the balances of the pool by exchanging large amounts of stable coins back and forth.
\end{itemize}

\subsection{Exploit Transaction Overview}
% add a graph
\begin{figure}[t]
  \centering
  \includegraphics[width=1.0\textwidth]{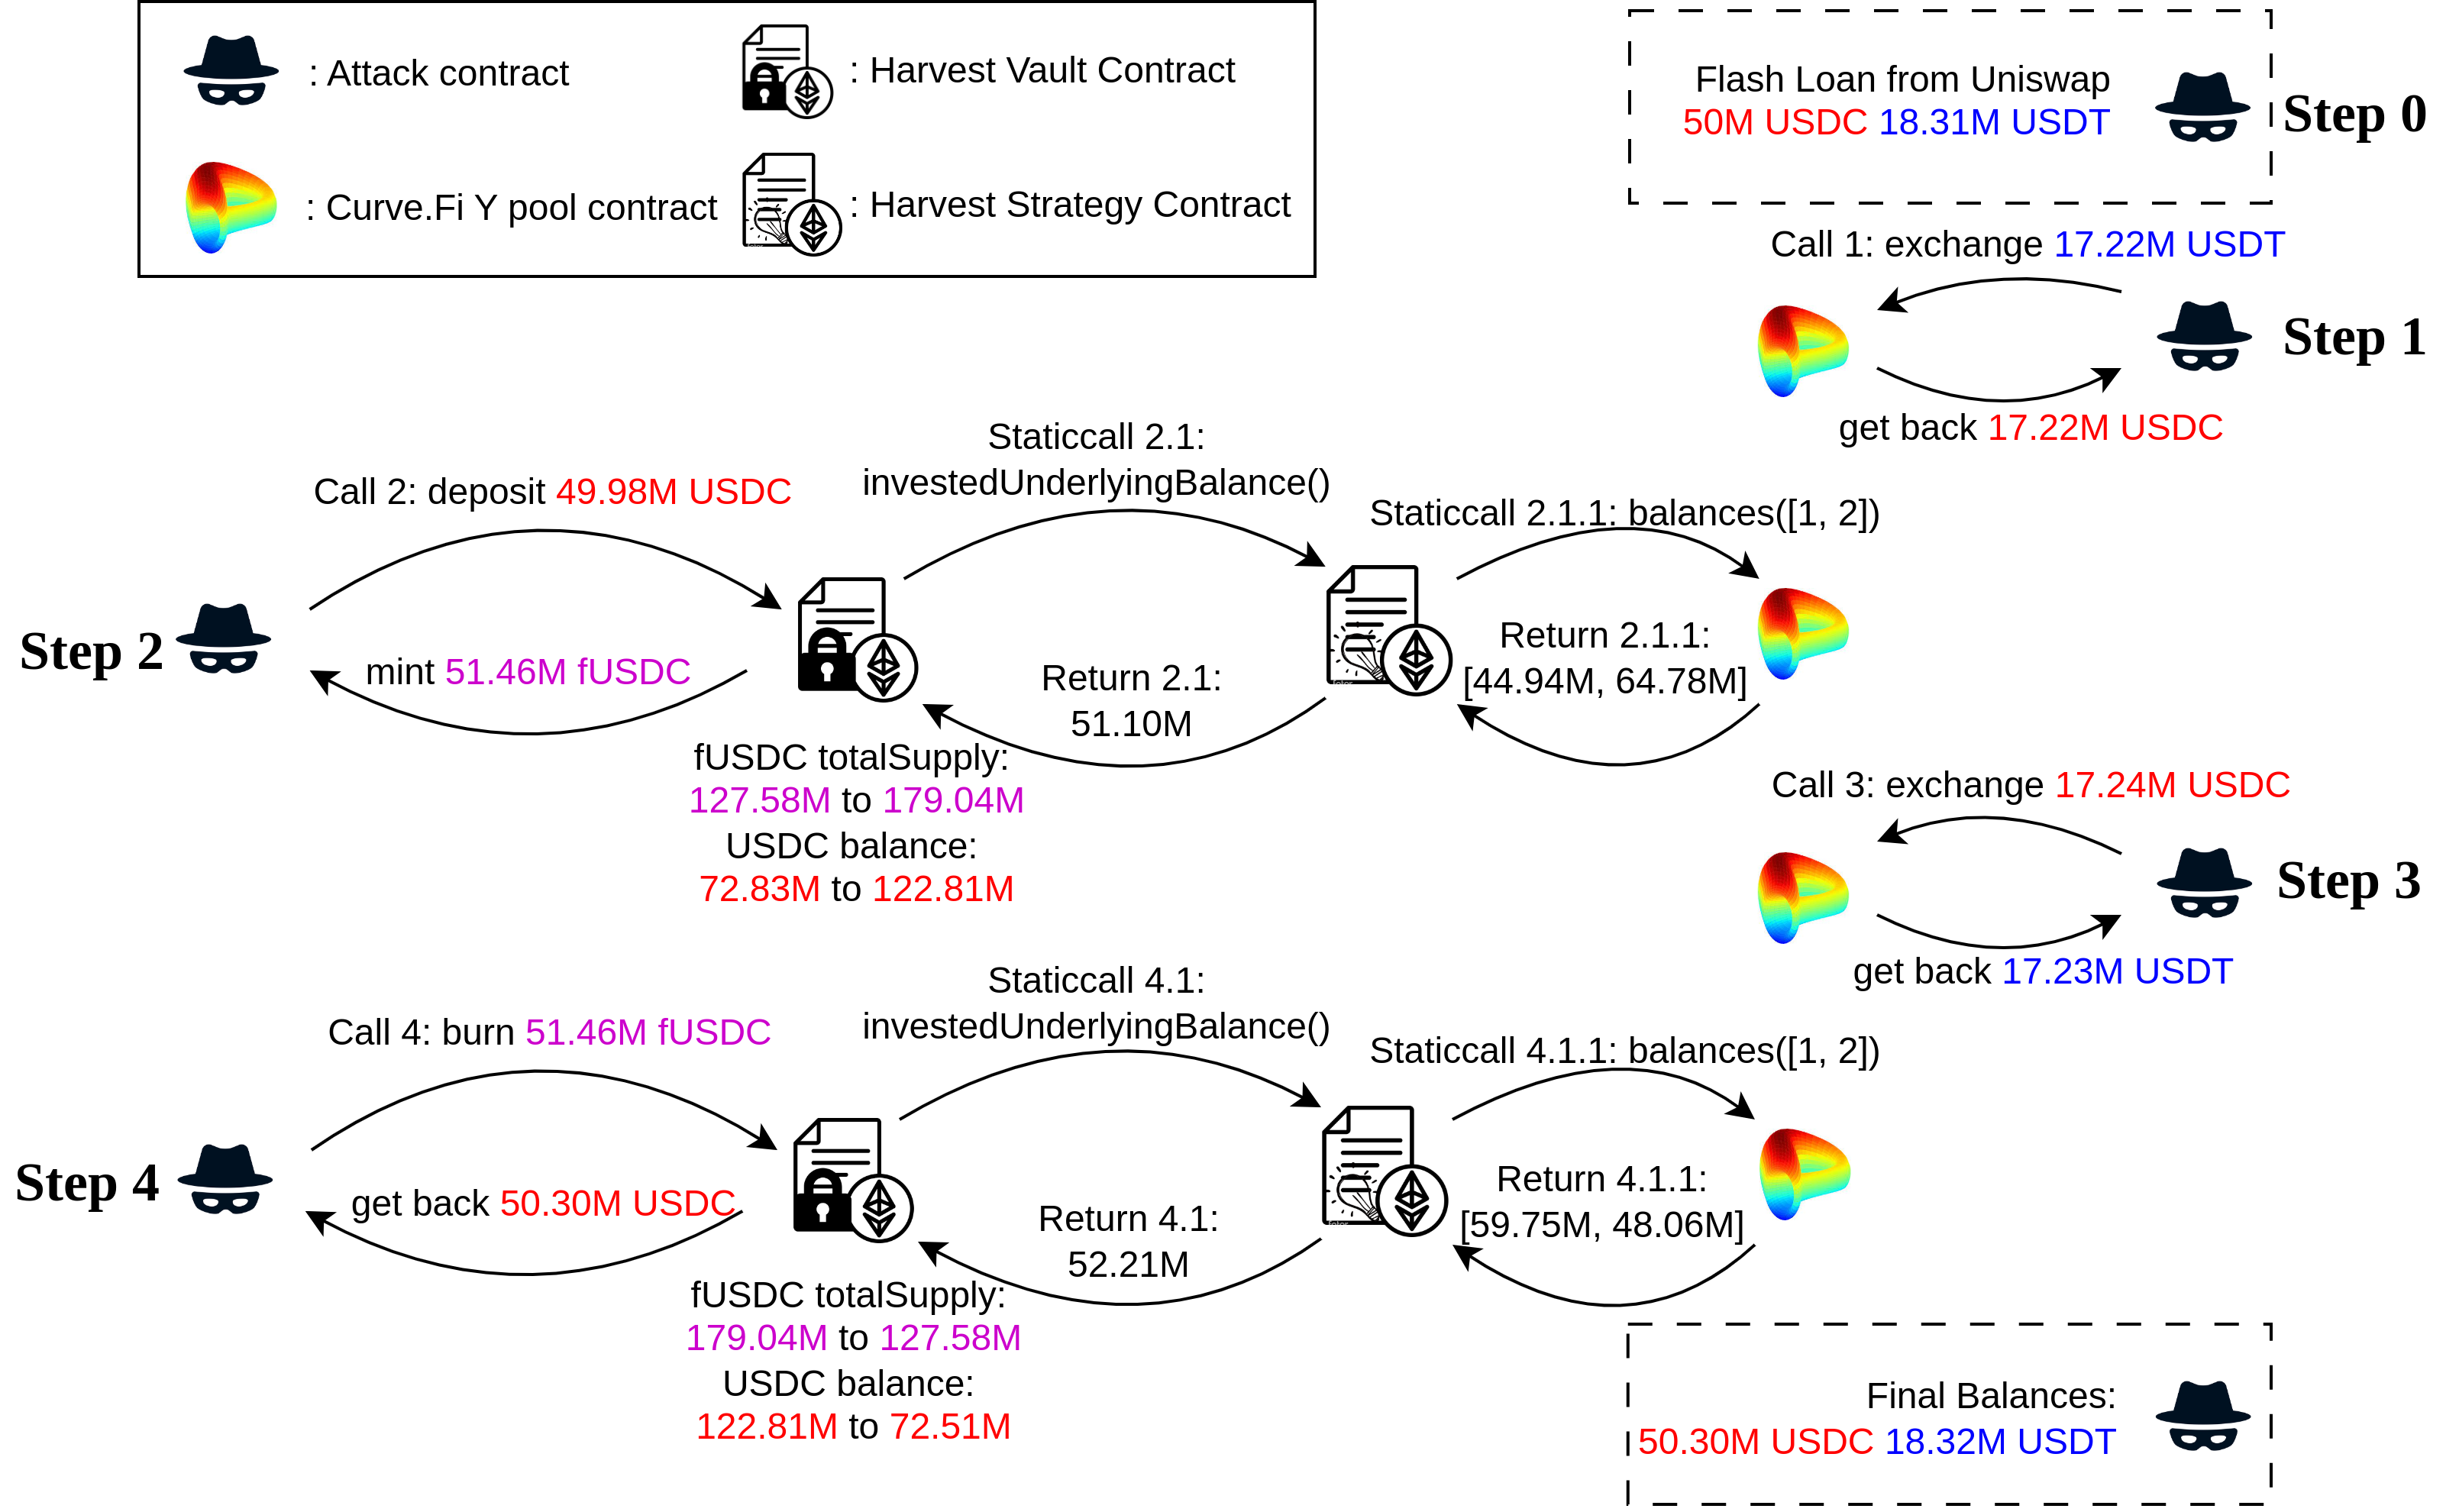}
  \caption{Harvest USDC Vault Attack Overview}
  \label{fig:harvest}
\end{figure}

The exploit transaction under consideration is complex, involving multiple steps and smart contract interactions. It starts with a flash loan of $50M$ USDC and $18.31M$ USDT from Uniswap, and proceeds to execute the same attack vector $3$ times. Figure~\ref{fig:harvest} summarizes the first attack vector, which interacts with Harvest vault contract and Curve.Fi Y pool contract, triggering a sequence of subsequent function calls. The transaction consumes abnormally $9,895,111$ gas, just within the gas limit of $12,065,986$ at the time.
The attack vector begins with an exchange of $17.22M$ USDT to $17.22M$ USDC via Curve.Fi Y pool contract. This exchange depletes the USDC balance and inflates the USDT balance in the Curve Y pool, leading to an underestimation of invested assets in the Harvest strategy contract, now valued at $51.10e12$.
Then the attack contract deposits $49.98$ USDC into Harvest vault contract, which increases its USDC balance from $72.83M$ to $122.51M$. Due to the underestimated value of invested assets, the attack contract receives an inflated $51.46M$ fUSDC back. This inflates the total fUSDC supply from $127.58M$ to $179.04M$.
The attack contract then reverses its initial exchange, converting $17.24M$ USDC back to $17.23M$ USDT, thereby restoring the original asset balances in the Curve Y pool.
In the final step, the attack contract redeems all its fUSDC tokens for $50.30M$ USDC, reducing the
Harvest vault's USDC balance from $122.81M$ to $72.51M$ and restoring the total fUSDC supply to its
original value of $127.58M$.
